# Supplementary material for: Privacy of Dependent Users Against Statistical Matching
Source: arXiv:1806.11108 source file (2019-05-29)
Supplement: Supplementary file 1 [file appendix_a.tex]

{\color{red}
\section{Discussion: More General Setting for Association Graph}
\label{appendixA}
In the community structure~\cite{Com1, Com2, Com3,Com4, Com5, Com_Negar}, the nodes of the network can be easily grouped into sets of users such that each set of users is densely connected internally according to Figure~\ref{graph1}. Here, we also assume that the adversary has some knowledge about all the covariance between users: he/she knows the value of the covariance is less than or higher than specific values. We show that the adversary can reliably reconstruct the entire association graph for \textit{the anonymized version of the data} (i.e., the observed data traces) with relatively few observations.

\begin{figure*}[t!]
	\centering
	\subfloat[A sketch of a small network displaying community structure.]{
		\includegraphics[width=0.5\columnwidth]{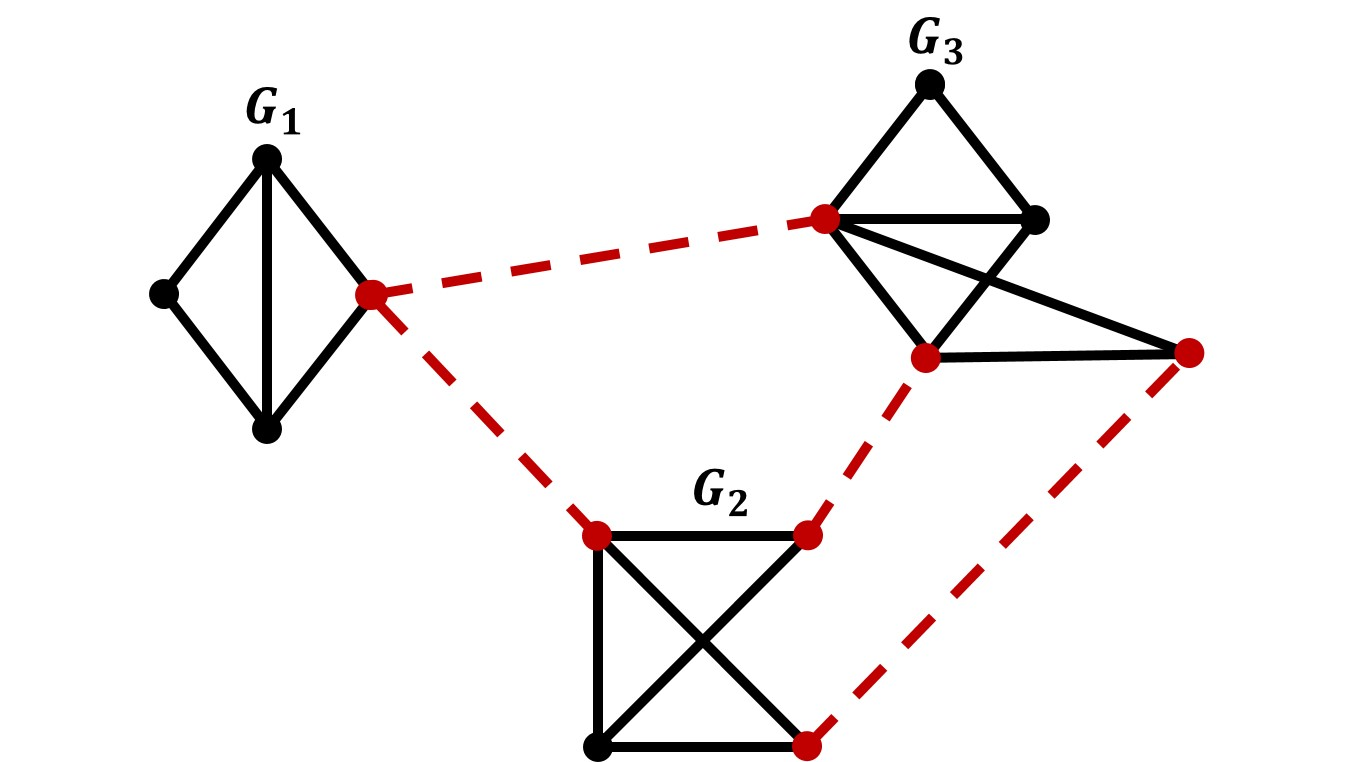}
		\label{fig:com1}
	}
	\subfloat[The association graph consists of disjoint subgraphs.]{
		\includegraphics[width=0.5\columnwidth]{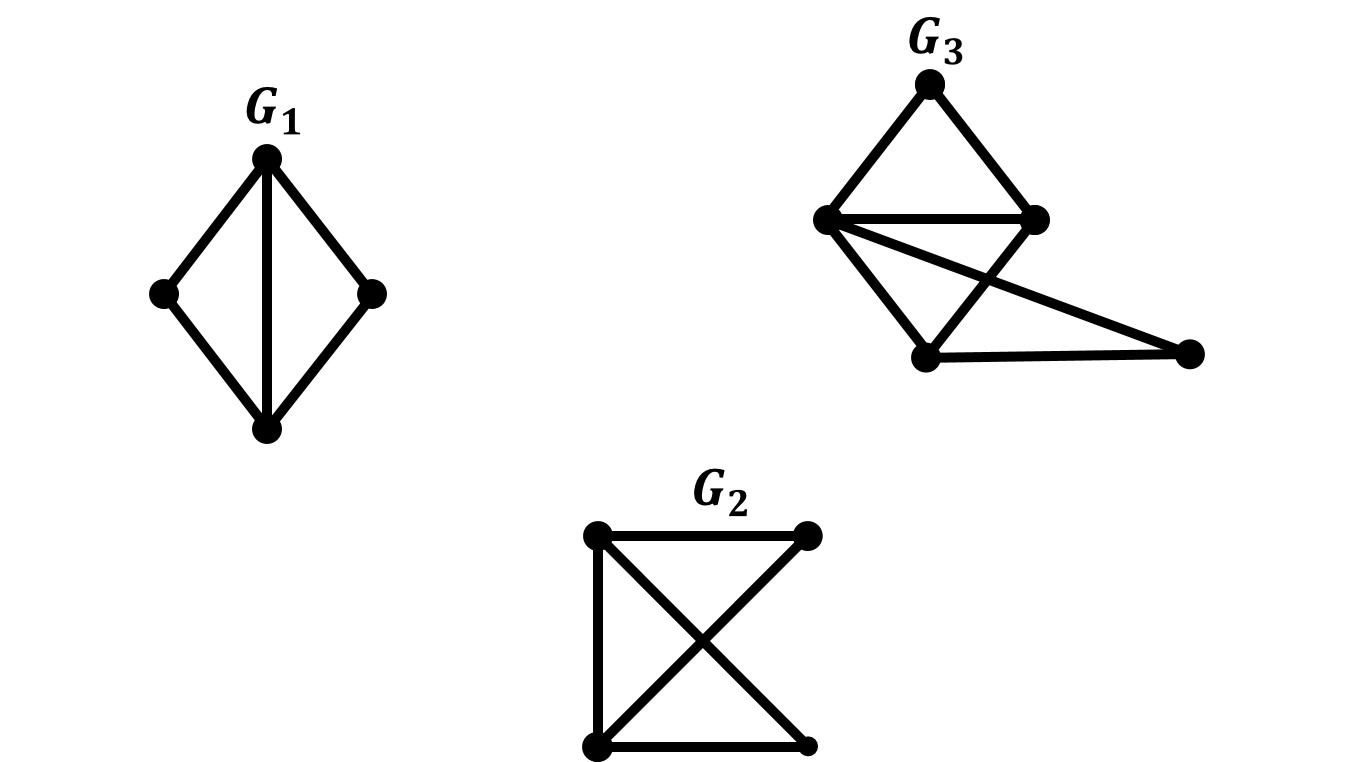}
		\label{fig:com2}
	}
	\caption{The adversary uses his/her prior knowledge to break inter-community edges.}
	\label{fig:com33}
\end{figure*}

\begin{lem}
	\label{lem3}
	Consider a general association graph $G(\mathcal{V},F)$. If the adversary obtains $m=(\log n)^3$ anonymized observations per user, he/she can construct $\widetilde{G}=\widetilde{G}(\widetilde{\mathcal{V}}, \widetilde{F})$, where $\widetilde{\mathcal{V}}=\{\Pi(u):u \in \mathcal{V}\}=\mathcal{V}$, such that with high probability, for all $u, u' \in \mathcal{V}$; $ (u,u')\in F$ iff $\left(\Pi(u),\Pi(u')\right)\in \widetilde{F}$. We write this statement as $\mathbb{P}(\widetilde{F}=F)\to 1$.
\end{lem}

\begin{proof}
	We provide an algorithm for the adversary that with high probability obtains all edges of $F$ correctly. For each pair $u$ and $u'$, compute
	\begin{align}
	\widetilde{Cov_{uu'}}&=\frac{\sum\limits_{i=1}^{r-1}\sum\limits_{i=1}^{r-1}ijM_{uu'}(i,j)}{m}-\frac{\sum\limits_{i=1}^{r-1}iM_{u}(i)}{m}\frac{\sum\limits_{i=1}^{r-1}iM_{u'}(i)}{m}\ \
	\label{cov}
	\end{align}
	where
	\[M_{uu'}(i,j)= \abs*{\left\{k: X_u(k)=i, X_{u'}(k)=j\right\}}.\]
	\[M_{u}(i)= \abs*{\left\{k: X_u(k)=i\right\}}.\]
	\[M_{u'}(i)= \abs*{\left\{k: X_{u'}(k)=i\right\}}.\]
	We claim for $m=\left(\log n\right)^3$,
	\begin{itemize}
		\item If $|\widetilde{Cov_{uu'}}|<\epsilon_1$, then $(u,u')\notin \widetilde{F}.$
		\item If $|\widetilde{Cov_{uu'}}|>\epsilon_2$, then $(u,u')\in \widetilde{F}.$
	\end{itemize}
	We show the above method yields $\mathbb{P}(\widetilde{F}=F)\to 1$ as $n \to \infty$, as follows.

	Note, according to (\ref{cov}), (\ref{M1}), (\ref{M2}), and (\ref{M3}),
	\begin{align}
	\no &\widetilde{Cov_{uu'}}=\frac{\sum\limits_{i=1}^{r-1}\sum\limits_{j=1}^{r-1}ijM_{uu'}(i,j)}{m}-\frac{\sum\limits_{i=1}^{r-1}iM_{u}(i)}{m}\frac{\sum\limits_{i=1}^{r-1}iM_{u'}(i)}{m}\\
	\no &\leq\frac{\sum\limits_{i=1}^{r-1}\sum\limits_{j=1}^{r-1}ij\left(mp_{uu'}(i,j)+m^{\frac{3}{4}}\right)}{m}-\frac{\sum\limits_{i=1}^{r-1}i\left(mp_{u}(i)-m^{\frac{3}{4}}\right)}{m}\frac{\sum\limits_{i=1}^{r-1}i\left(mp_{u'}(i)-m^{\frac{3}{4}}\right)}{m}\\
	\no&= \sum\limits_{i=1}^{r-1}\sum\limits_{j=1}^{r-1}ij p_{uu'}(i,j)-\sum\limits_{i=1}^{r-1}ip_u(i)\sum\limits_{i=1}^{r-1}ip_{u'}(i)+\frac{r(r-1)}{2}m^{-\frac{1}{4}}+\frac{r(r-1)}{2} \sum\limits_{i=1}^{r-1}i(p_u(i)+p_{u'}(i))m^{-\frac{1}{4}}\\
	&= \rho_{uu'}\sigma_u \sigma_{u'}+O(m^{-\frac{1}{4}}).\ \
	\label{eq1}
	\end{align}
	Similarly,
	\begin{align}
	\no &\widetilde{Cov_{uu'}}=\frac{\sum\limits_{i=1}^{r-1}\sum\limits_{j=1}^{r-1}iM_{uu'}(i,j)}{m}-\frac{\sum\limits_{i=1}^{r-1}iM_{u}(i)}{m}\frac{\sum\limits_{i=1}^{r-1}iM_{u'}(i)}{m}\\
	\no &\geq\frac{\sum\limits_{i=1}^{r-1}i\left(mp_{u}(i)-m^{\frac{3}{4}}\right)}{m}-\frac{\sum\limits_{i=1}^{r-1}i\left(mp_{u}(i)+m^{\frac{3}{4}}\right)}{m}\frac{\sum\limits_{i=1}^{r-1}i\left(mp_{u'}(i)+m^{\frac{3}{4}}\right)}{m}\\
	&= \rho_{uu'}\sigma_u \sigma_{u'}-O(m^{-\frac{1}{4}}).\ \
	\label{eq2}
	\end{align}
	Now, by using (\ref{eq1}) and (\ref{eq2}), we have
	\begin{align}
	\mathbb{P}\left(\abs*{\widetilde{Cov_{uu'}}-Cov_{uu'}} \leq m^{-\frac{1}{5}}\right) \to 1,\ \
	\label{cov1}
	\end{align}	
	thus, we can conclude for all $u,u' \in\{1, 2, \cdots, n\}$, $\widetilde{Cov_{uu'}}$'s are close to $Cov_{uu'}$'s.
	Now, for all inter-community edges, the adversary knows $Cov_{uu'} \leq \epsilon_1$, so we can conclude $\widetilde{Cov_{uu'}} \leq \epsilon_1$ with high probability and as a result the adversary remove that edge. In addition, for all intra-community edges, the adversary knows $Cov_{uu'} \geq \epsilon_2$, so we can conclude $\widetilde{Cov_{uu'}} \geq \epsilon_2$ with high probability.
%	For $(u,u') \notin F$, we have $\rho_{uu'}=0$, thus, by using (\ref{eq1}) and (\ref{eq2}), with high probability, we have
%	\begin{align}
%	\no |\widetilde{Cov_{uu'}}|\leq O(m^{-\frac{1}{4}}), \ \ \ \textrm{for all }u,u' \in \{1,2,\cdots, n\}.\ \
%	\end{align}
%	Then, as $n \to \infty$,
%	\begin{align}
%	\no \mathbb{P}\left(|\widetilde{Cov_{uu'}}|\leq m^{-\frac{1}{5}}\right)\to 1.
%	\end{align}
%	
%	Similarly, for $(u,u') \in F$, we have $\rho_{uu'} \neq 0$, thus, by using (\ref{eq1}) and (\ref{eq2}), we have
%	\begin{align}
%	\no \widetilde{Cov_{uu'}}\leq  \rho_{uu'}\sigma_u \sigma_{u'}+O(m^{-\frac{1}{4}}),  \  \rho_{uu'}\sigma_u \sigma_{u'}\neq 0,\ \
%	\end{align}
%	and
%	\begin{align}
%	\no \widetilde{Cov_{uu'}}\geq  \rho_{uu'}\sqrt{\sigma^2_u \sigma^2_{u'}}-O(m^{-\frac{1}{4}}),  \  \rho_{uu'}\sigma_u \sigma_{u'} \neq 0,\ \
%	\end{align}
%	and as a result, as $n \to \infty,$
%	\begin{align}
%	\no \mathbb{P}\left(|\widetilde{Cov_{uu'}}|\geq m^{-\frac{1}{5}}\right)\to 1.
%	\end{align}
	
	As a result, for large enough $n$, we have $\mathbb{P}\left(\widetilde{F}=F\right)\to 1$, so the adversary can reconstruct the association graph of the anonymized version of the data with arbitrarily small error probability. 
\end{proof}

Now, the adversary have a graph structure shown in Figure \ref{fig:com2}, where the association graph consists of $f$ disjoint subgraphs,
\[G=G_1 \cup G_2 \cup \cdots \cup  G_f,\]
where subgraph $G_l$ is a connected graph on $s_l$ vertices.

%
%
%The structure of the association graph $(G)$ can leak a lot of information. For example, in Figure \ref{fig:identity}, the identity map is the only automorphism of the association graph $G$. Thus, it is obvious that the adversary can uniquely identify all of the users if he/she can reconstruct the association graph $\widetilde{G}$ of the anonymized data.

%For the rest of the paper, we consider a graph structure shown in Figure \ref{fig:graph}, where the association graph consists of $f$ disjoint subgraphs,
%\[G=G_1 \cup G_2 \cup \cdots \cup  G_f,\]
%where subgraph $G_l$ is a connected graph on $s_l$ vertices. In particular, each subgraph $G_l$ can be thought of as a group of ``friends'' or ``associates'' such that their data sets are dependent. So, we can write $G_l(\mathcal{V}_l, F_l)$, where $|\mathcal{V}_l|=s_l$. Note that, we assume $s_l$'s are finite.
%
%\begin{figure}
%	\centering
%	\includegraphics[width=.4\linewidth]{fig/identity.jpg}
%	\centering
%	\caption{One example of an association graph for which the identity map is the only automorphism.}
%	\label{fig:identity}
%\end{figure}
%
%\begin{figure}
%	\centering
%	\includegraphics[width=.5\linewidth]{fig/graph.jpg}
%	\centering
%	\caption{The association graph $G$ consists of a collection of disjoint subgraphs $(G_l)$, where $G_l$ is a connected graph on $s_l$ vertices.}
%	\label{fig:graph}
%\end{figure}

}
